# Supplementary material for: See & Sniff: Learning Visuo-Olfactory Representations
Source: arXiv:2606.27307 source file (2026-06-25)
Supplement: Supplementary file 1 [file Suppl_data_distribution.tex]

\begin{table}[!t]
\centering
\small
\setlength{\tabcolsep}{8pt}
\resizebox{0.65\columnwidth}{!}{
\begin{tabular}{l|l|r|r|r}
\toprule
\textbf{Family} & \textbf{Ingredient} & \textbf{Train} & \textbf{Test-S} & \textbf{Test-IS} \\
\midrule

\multirow{10}{*}{Fruits}
& Apple & 581 & 20 & 4 \\
& Banana & 588 & 20 & 4 \\
& Kiwi & 581 & 20 & 4 \\
& Lemon & 538 & 20 & 4 \\
& Mango & 249 & 20 & 4 \\
& Mandarin\_Orange & 312 & 20 & 4 \\
& Peach & 278 & 20 & 4 \\
& Pear & 261 & 20 & 4 \\
& Pineapple & 259 & 20 & 4 \\
& Strawberry & 248 & 20 & 4 \\
\midrule

\multirow{10}{*}{Herbs}
& Angelica & 204 & 20 & 3 \\
& Chamomile & 288 & 20 & 4 \\
& Chives & 245 & 20 & 4 \\
& Coriander & 282 & 20 & 4 \\
& Dill & 230 & 20 & 4 \\
& Garlic & 254 & 20 & 4 \\
& Mint & 250 & 20 & 4 \\
& Mugwort & 256 & 20 & 4 \\
& Oregano & 274 & 20 & 4 \\
& Turnip & 261 & 20 & 4 \\
\midrule

\multirow{10}{*}{Nuts}
& Almond & 269 & 20 & 4 \\
& Brazil\_Nut & 271 & 20 & 4 \\
& Cashew & 252 & 20 & 4 \\
& Chestnuts & 251 & 20 & 4 \\
& Hazelnut & 262 & 20 & 4 \\
& Peanuts & 255 & 20 & 4 \\
& Pecans & 250 & 20 & 4 \\
& Pili\_Nut & 224 & 20 & 3 \\
& Pistachios & 251 & 20 & 4 \\
& Walnuts & 252 & 20 & 4 \\
\midrule

\multirow{10}{*}{Spices}
& Allspice & 313 & 20 & 4 \\
& Chervil & 254 & 20 & 4 \\
& Cinnamon & 315 & 20 & 4 \\
& Cloves & 317 & 20 & 4 \\
& Cumin & 363 & 20 & 4 \\
& Ginger & 358 & 20 & 4 \\
& Mustard & 341 & 20 & 4 \\
& Nutmeg & 323 & 20 & 4 \\
& Saffron & 309 & 20 & 4 \\
& Star\_Anise & 312 & 20 & 4 \\
\midrule

\multirow{10}{*}{Vegetables}
& Asparagus & 262 & 20 & 4 \\
& Avocado & 256 & 20 & 4 \\
& Broccoli & 252 & 20 & 4 \\
& Brussel\_Sprouts & 250 & 20 & 4 \\
& Cabbage & 272 & 20 & 5 \\
& Cauliflower & 259 & 20 & 4 \\
& Potato & 249 & 20 & 4 \\
& Radish & 367 & 20 & 4 \\
& Sweet\_Potato & 563 & 20 & 4 \\
& Tomato & 583 & 20 & 5 \\
\midrule

\textbf{Total}& & \textbf{15,494} & \textbf{1,000} & \textbf{200} \\
\bottomrule
\end{tabular}
}
\caption{Ingredient-wise image distribution in the train set and the Source(Test-S) and InteractiveSource(Test-IS) test sets of SmellNet-V.}
\label{tab:data_distribution}
\end{table}
